# Supplementary material for: Random Walk Guided Hyperbolic Graph Distillation
Source: arXiv:2501.15696 source file (2025-01-26)
Supplement: Supplementary file 1 [file data_statistics.tex]

\begin{table}[h]
\centering
\caption{Dataset statics, including five node classification datasets, two anomaly detection datasets, and two link prediction datasets.}
\label{tab:dataset_statics}
\begin{tabular}{llrrrr}
\hline
 & \textbf{Datasets} & \multicolumn{1}{l}{\textbf{\#Nodes}} & \multicolumn{1}{l}{\textbf{\#Edges}} & \multicolumn{1}{l}{\textbf{\#Classes}} & \multicolumn{1}{l}{\textbf{\#Features}} \\ \hline
\multirow{5}{*}{\textbf{ND}} & Cora~\cite{kipf2016semi}  & 2,708 & 5,429 & 7 & 1,433 \\
 & Citeseer~\cite{kipf2016semi} & 3,327 & 4,732 & 6 & 3,703 \\
 & Ogbn-arxiv~\cite{hu2020open} & 169,343 & 1,166,243 & 40 & 128 \\
 & Flickr~\cite{graphsaint-iclr20} & 89,250 & 899,756 & 7 & 500 \\
 & Reddit~\cite{hamilton2017inductive} & 232,965 & 57,307,946 & 210 & 602 \\ \hline
\multirow{2}{*}{\textbf{AD}} & YelpChi~\cite{yelpChi} & 45,954 & 3,846,979 & 2 & 32 \\
 & Amazon~\cite{Amazon} & 11,944 & 4,398,392 & 2 & 25 \\ \hline
\multirow{2}{*}{\textbf{LP}} & Citeseer-L~\cite{kipf2016semi} & 3,327 & 4,732 & 2 & 3,703 \\
 & DBLP~\cite{DBLP} & 26,128 & 105,734 & 2 & 4,057 \\ \hline
\end{tabular}
\end{table}
